# Supplementary material for: Excitation and detection of short-waved spin waves in ultrathin Ta/CoFeB/MgO-layer system suitable for spin-orbit-torque magnonics
Source: arXiv:1701.01399 ancillary file (2017-01-05)
Supplement: Supplementary file 1 [file Supplement.pdf]

# Supplementary material: Excitation and detection of short-waved spin waves in ultrathin Ta/CoFeB/MgO-layer system suitable for spin-orbit-torque magnonics

For an extension of the analytical formalism presented in Ref. 1, we follow the implementation of perpendicular magnetic anisotropy (PMA) discussed in Ref. 2. The dispersion relation for an ultra-thin, in-plane magnetized waveguide in the absence of interfacial Dzyaloshinskii-Moriya interaction and in-plane anisotropies can be approximated by

$$f(\mathbf{k}) = \sqrt{(\omega_0 + \omega_\mathrm{M}\lambda_\mathrm{ex}\mathbf{k}^2)(\omega_0 + \omega_\mathrm{M}\lambda_\mathrm{ex}\mathbf{k}^2 + (\omega_\mathrm{M} - \omega_\mathrm{Hu})F_{00}(\mathbf{k}))}. \tag{S1}$$

Here, $\gamma$ is the gyromagnetic ratio in units of $\mathrm{GHz\,T^{-1}}$ and $\mathbf{k}$ is the spin-wave wave vector. $\omega_0 = \gamma\mu_0 H_\mathrm{eff}$ with the effective field $H_\mathrm{eff}$ which accounts for the demagnetization field of the waveguide, $\omega_\mathrm{M} = \gamma\mu_0 M_\mathrm{s}$ with the saturation magnetization $M_\mathrm{s}$. $\lambda_\mathrm{ex} = 2A_\mathrm{ex}/(\mu_0 M_\mathrm{s}^2)$, where $A_\mathrm{ex}$ is the exchange constant. $\omega_\mathrm{Hu} = \gamma\mu_0 H_\perp = 4\gamma\mu_0 K_\perp/(M_\mathrm{s}\cdot d)$ with the out-of-plane anisotropy field $H_\perp$, the PMA constant $K_\perp$ and the thickness $d$ of the ferromagnetic layer. $F_{00}(\mathbf{k})$ is given by

$$F_{00}(\mathbf{k}) = 1 + g(\mathbf{k})(\sin(\theta_k)^2 - 1) + \frac{\omega_\mathrm{M} g(\mathbf{k})(1 - g(\mathbf{k}))\sin(\theta_k)^2}{\omega_0 + \omega_\mathrm{M}\lambda_\mathrm{ex}\mathbf{k}^2}, \tag{S2}$$

where $\theta_k$ is the angle between the spin-wave wave vector and the magnetization. $g(\mathbf{k}) = 1 - (1 - \exp(|\mathbf{k}|d))/(|\mathbf{k}|d)$.

Figure S1 shows a set of dispersion relations for different PMA constants $K_\perp$ calculated via Eq. S1 together with the dispersion relations obtained from numerical simulations using MuMax3[3]. To obtain the dispersion from the simulation, $w = 1\,\mu$m wide, $L = 10\,\mu$m long and $d = 1.4$ nm thick CoFeB waveguides with identical material parameters than in the analytical calculations (i.e. $M_\mathrm{s} = 1250\,\mathrm{kA\,m^{-1}}$, $A_\mathrm{ex} = 13\,\mathrm{pJ\,m^{-1}}$, anisotropy constants $K_\perp$ as indicated in the figure legend, $\gamma = 28\,\mathrm{GHz\,T^{-1}}$) have been discretized into $2048\times256\times1$ cells (length×width×thickness). The magnetization is excited by a Gaussian excitation pulse with a width of 20 ps in a rectangular area in the center of the waveguide ($10 \times 1000$ nm). The evolution of the magnetization after this excitation is simulated over a total time of 20 ns and the magnetization is saved as a function of space every 20 ps. The resulting data are transformed into the frequency-wave-vector domain via two subsequent Fast Fourier transformations. From these transformed data, the spin-wave dispersion relation of the fundamental mode is extracted.

As can be seen from Fig. S1 (a), the analytical approximation leads to a decent prediction of the spin-wave dispersion. Only at large values of $K_\perp$ close to the transition from in-plane to out-of-plane, a notable discrepancy between the approximation and the numerical simulation is found. In particular, for an anisotropy constant of $K_\perp = 0.6125\,\mathrm{mJ\,m^{-2}}$, a value close to the value observed in the experiment, the discrepancy between Eq. S1 and the simulation is below 4 % at the largest experimentally observed wave vector in the manuscript. Consequently, Eq. S1 is sufficiently precise to describe the experimentally observed spectra.

From the dispersion relation, the spin-wave group velocity $v_\mathrm{g}$ can be obtained via a simple derivation with respect to the wave vector $\mathbf{k}$. The spin-wave lifetime can be approximated via[1,4]

$$\tau = \left(\alpha\omega(\mathbf{k})\frac{\partial\omega(\mathbf{k})}{\partial\omega_0}\right)^{-1} = \left(2\pi\alpha\left(\omega_0 + \omega_\mathrm{M}\lambda_\mathrm{ex}\mathbf{k}^2 + \frac{(\omega_\mathrm{M} - \omega_\mathrm{Hu})(1 + g(\mathbf{k}))(\sin(\theta_k)^2 - 1)}{2}\right)\right)^{-1}. \tag{S3}$$

Here, $\omega(\mathbf{k}) = 2\pi f(\mathbf{k})$ and $\alpha$ is the Gilbert damping parameter. Evidently, the PMA reduces also the ellipticity

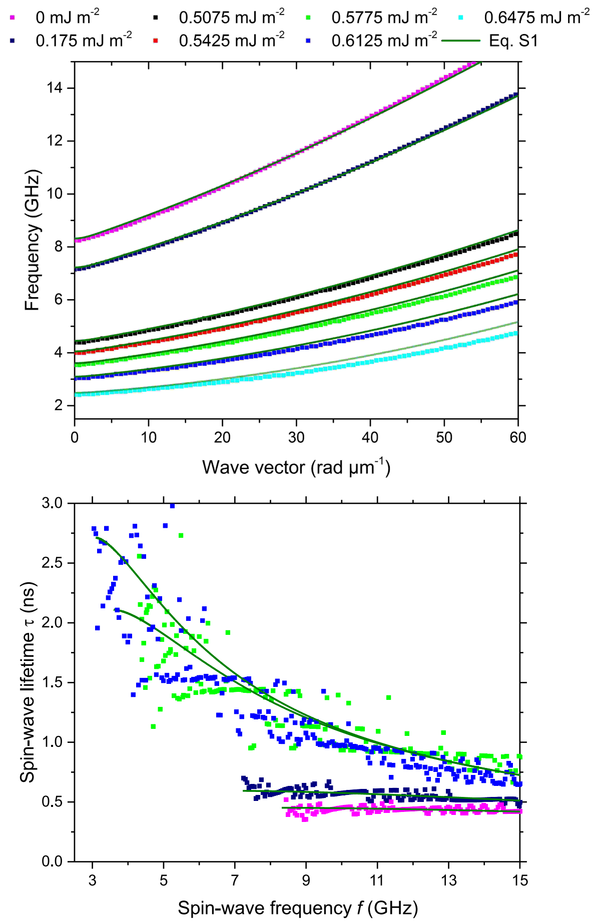


FIG. S1. a) Squares: Numerically simulated dispersion relation in a 1 $\mu$m wide and 1.4 nm thick CoFeB waveguide for different perpendicular magnetic anisotropy constants $K_\perp$. Solid lines: Approximated dispersion from Eq. S1 with the corresponding anisotropy constants $K_\perp$ given in the figure legend. b) Corresponding spin-wave lifetimes $\tau$ obtained from the micromagnetic simulations (squares) and according to Eq. S3.

contribution to the spin-wave relaxation, which is given by the fractional term in Eq. S3. Similar to the arguments for the ferromagnetic resonance in the manuscript, this results in a significant enhancement of the spin-wave lifetime, since $\omega_\mathrm{M} \gg \omega_0$. This can be comprehended from Fig. S1 (b), where the spin-wave lifetime $\tau$ is shown as a function of frequency for several exemplary values of $K_\perp$. The solid lines are calculated according to Eq. S3 and the squares are extracted from the numerical simulations. For this extraction, the spin-wave decay is fitted in the frequency-space-domain as described in Ref. 1 and the spin-wave amplitude decay length $\delta = v_\mathrm{g}\tau$ is extracted from this exponential fit. The values of the decay length are consequently divided by the spin-wave group velocity $v_\mathrm{g}$, which has been obtained from the derivative of the numerically simulated dispersion relation. As can be seen from the figure, the PMA leads to a significant enhancement of the lifetime, in particular for small frequencies. The lifetime predicted by Eq. S3 is in good quantitative agreement with these findings. The observed values beyond 2 ns are remarkably large and, as stated in the manuscript, even exceed the spin-wave lifetime in thicker films in common materials like $\mathrm{Ni_{81}Fe_{19}}$ ($\alpha \approx 0.008$), despite the presence of interfacial damping in the ultrathin CoFeB films ($\alpha = 0.015$). This shows the important contribution of the ellipticity of precession on the spin-wave lifetime in thin films.

As discussed in the manuscript, the PMA also influences the asymmetry of the CPW excitation since it decreases the ellipticity of precession. This way, it increases the excitation efficiency of the out-of-plane component of the field created by the CPW and increases the interplay between the dynamic magnetization components in- and out-of-plane. In the presence of PMA, the expression for the excitation efficiency in a transversely magnetized waveguide in Ref. 1 is modified to

$$\eta_\pm(k_\pm) = \left| \frac{1}{n} |b_k| \left( \frac{f(k_\pm)}{\gamma} \mp \frac{1}{\mu_0(M_\mathrm{s} - H_\perp)} \left( \mu_0 H_\mathrm{eff}^2 - \frac{f(k_\pm)^2}{\gamma^2} \right) \right) \right| . \tag{S4}$$

Here, $k_\pm$ and the $\pm$ in the equation refer to waves running to the left and waves running to the right from the excitation source. $|b_k|$ represents the Fourier transform of the field distribution of the excitation source. The effective reduction of the saturation magnetization in the last term of the equation is responsible for the strong asymmetry.


[1] T. Brächer, P. Pirro, O. Boulle, and G. Gaudin, *Creation of unidirectional spin-wave emitters by utilizing interfacial Dzyaloshinskii-Moriya interaction*, Wonderful journal of astonishing physics **1**, 2016.

[2] J. A. C. Bland, B. Heinrich, *Ultrathin Magnetic Structures II*, Springer-Verlag Berlin Heidelberg (1994).

[3] A. Vansteenkiste, J. Leliaert, M. Dvornik, M. Helsen, F. Garcia-Sanchez, and B. Van Waeyenberge, *The design and verification of mumax3*, AIP Advances **4**, 107133 (2014).

[4] D. D. Stancil and A. Prabhakar, *Spin Waves, Theory and Applications*, Springer (2009).
